# Supplementary material for: SoK: DARPA's AI Cyber Challenge (AIxCC): Competition Design, Architectures, and Lessons Learned
Source: arXiv:2602.07666 source file (2026-08-02)
Supplement: Supplementary file 1 [file appendix_cp_table.tex]

\begin{table*}[t]
\centering
\caption{Detailed information about each challenge project (CP)
in the AIxCC final round.
$\square$: full-mode; $\blacktriangle$: delta-mode.
Cutoff: date of the latest upstream commit
incorporated into the organizer's CP repository.
$\dagger$: measured on AMD EPYC 7452 (128 cores), 512\,GB RAM, Ubuntu 22.04.}
\label{t:cp-details}
\smaller
\setlength{\tabcolsep}{3pt}
\adjustbox{max width=\textwidth}{
\begin{threeparttable}
\begin{tabular}{@{}>{\cellcolor{white}}l >{\cellcolor{white}}l >{\cellcolor{white}}l >{\cellcolor{white}}r l r l r r r r r r r@{}}
\toprule
\textbf{Lang.} & \textbf{Project} & \textbf{Category} & \textbf{\# Harn.} & \textbf{CP} & \textbf{\# CPVs} & \textbf{CWEs} & \textbf{SLOC} & \textbf{Commit} & \textbf{Cutoff} & \textbf{$\Delta$ Lines} & \textbf{$\Delta$ Files} & \shortstack[c]{\textbf{Build}\\\textbf{Time}$^\dagger$} & \shortstack[c]{\textbf{Harn.}\\\textbf{Size}} \\
\midrule
 &  &  &  & \cc{cu2$\blacktriangle$} & 1 & \href{https://cwe.mitre.org/data/definitions/476.html}{476} & 238K & \href{https://github.com/curl/curl/commit/2d4852af8}{\cc{2d4852a}} & 2024-12-09 & 881 & 24 & 110s & 232.6MB \\
\rowcolor{gray!15}  &  &  &  & \cc{cu3$\blacktriangle$} & 1 & \href{https://cwe.mitre.org/data/definitions/476.html}{476} & 238K & \href{https://github.com/curl/curl/commit/2d4852af8}{\cc{2d4852a}} & 2024-12-09 & 940 & 25 & 112s & 232.8MB \\
 &  &  &  & \cc{cu4$\blacktriangle$} & 2 & \href{https://cwe.mitre.org/data/definitions/121.html}{121}, \href{https://cwe.mitre.org/data/definitions/476.html}{476} & 238K & \href{https://github.com/curl/curl/commit/2d4852af8}{\cc{2d4852a}} & 2024-12-09 & 1,252 & 33 & 109s & 232.8MB \\
\rowcolor{gray!15}  &  &  &  & \cc{cu5$\blacktriangle$} & 2 & \href{https://cwe.mitre.org/data/definitions/134.html}{134}, \href{https://cwe.mitre.org/data/definitions/787.html}{787} & 237K & \href{https://github.com/curl/curl/commit/2d4852af8}{\cc{2d4852a}} & 2024-12-09 & 657 & 27 & 112s & 232.3MB \\
 & \multirow{-5}{*}{\href{https://github.com/curl/curl}{curl}} & \multirow{-5}{*}{Network} & \multirow{-5}{*}{17} & \cc{cu6$\blacktriangle$} & 0 & -- & 249K & \href{https://github.com/curl/curl/commit/4dacb79fc}{\cc{4dacb79}} & 2025-05-28 & 51,469 & 1,132 & 125s & 238.0MB \\
\cmidrule{2-14}
\rowcolor{gray!15}  & \href{https://github.com/videolan/dav1d}{dav1d} & Codec & 1 & \cc{da1$\square$} & 1 & \href{https://cwe.mitre.org/data/definitions/190.html}{190} & 261K & \href{https://github.com/videolan/dav1d/commit/08051a3b50dee91a88e2bff0391c5abd89da1c12}{\cc{08051a3}} & 2024-02-06 & -- & -- & 38s & 910B \\
\cmidrule{2-14}
 &  &  &  & \cc{fp2$\blacktriangle$} & 1 & \href{https://cwe.mitre.org/data/definitions/122.html}{122} & 453K & \href{https://github.com/FreeRDP/FreeRDP/commit/f1285ade4607527576e8438e724e13b8a3ff6807}{\cc{f1285ad}} & 2025-02-11 & 373 & 10 & 205s & 190.6MB \\
\rowcolor{gray!15}  &  &  &  & \cc{fp3$\blacktriangle$} & 1 & \href{https://cwe.mitre.org/data/definitions/123.html}{123} & 453K & \href{https://github.com/FreeRDP/FreeRDP/commit/f1285ade4607527576e8438e724e13b8a3ff6807}{\cc{f1285ad}} & 2025-02-11 & 498 & 10 & 209s & 190.6MB \\
 & \multirow{-3}{*}{\href{https://github.com/FreeRDP/FreeRDP}{freerdp}} & \multirow{-3}{*}{Remote Desktop} & \multirow{-3}{*}{7} & \cc{fp4$\blacktriangle$} & 0 & -- & 463K & \href{https://github.com/FreeRDP/FreeRDP/commit/fcdf4c6c7e7ffda9203889114a2ee7ba8d5d1976}{\cc{fcdf4c6}} & 2025-06-16 & 20,605 & 256 & 207s & 190.5MB \\
\cmidrule{2-14}
\rowcolor{gray!15}  &  &  &  & \cc{av2$\blacktriangle$} & 1 & \href{https://cwe.mitre.org/data/definitions/126.html}{126} & 44K & \href{https://github.com/AOMediaCodec/libavif/commit/fa089a0c3f8ed6e202034589cf98394e0226d66c}{\cc{fa089a0}} & 2025-04-14 & 1,407 & 25 & 168s & 50.8MB \\
 & \multirow{-2}{*}{\href{https://github.com/AOMediaCodec/libavif}{libavif}} & \multirow{-2}{*}{Image} & \multirow{-2}{*}{8} & \cc{av3$\blacktriangle$} & 0 & -- & 44K & \href{https://github.com/AOMediaCodec/libavif/commit/1aadfad932c98c069a1204261b1856f81f3bc199}{\cc{1aadfad}} & 2025-05-09 & 3,232 & 98 & 207s & 2.4KB \\
\cmidrule{2-14}
\rowcolor{gray!15}  &  &  &  & \cc{ex2$\blacktriangle$} & 1 & \href{https://cwe.mitre.org/data/definitions/122.html}{122} & 16K & \href{https://github.com/libexif/libexif/commit/30e50906596aa69a484c1044abb07eaa0ffda2dd}{\cc{30e5090}} & 2022-04-21 & 210 & 12 & 49s & 11.6MB \\
 & \multirow{-2}{*}{\href{https://github.com/libexif/libexif}{libexif}} & \multirow{-2}{*}{Image} & \multirow{-2}{*}{2} & \cc{ex3$\blacktriangle$} & 1 & \href{https://cwe.mitre.org/data/definitions/121.html}{121} & 15K & \href{https://github.com/libexif/libexif/commit/a918830b8830e1e3657b4f36f48571a8d95a4ec8}{\cc{a918830}} & 2021-11-01 & 178 & 9 & 50s & 11.7MB \\
\cmidrule{2-14}
\rowcolor{gray!15}  & \href{https://github.com/GNOME/libxml2}{libxml2} & Document & 11 & \cc{lx3$\blacktriangle$} & 1 & \href{https://cwe.mitre.org/data/definitions/122.html}{122} & 201K & \href{https://github.com/GNOME/libxml2/commit/71c37a565d3726440aa96d648db0426deb90157b}{\cc{71c37a5}} & 2024-12-30 & 634 & 13 & 58s & 136.3MB \\
\cmidrule{2-14}
 &  &  &  & \cc{cm1$\blacktriangle$} & 0 & -- & 87K & \href{https://github.com/mm2/Little-CMS/commit/5176347635785e53ee5cee92328f76fda766ecc6}{\cc{5176347}} & 2025-02-04 & 8,072 & 140 & 33s & 93.0MB \\
\rowcolor{gray!15}  & \multirow{-2}{*}{\href{https://github.com/mm2/Little-CMS}{little-cms}} & \multirow{-2}{*}{Image} & \multirow{-2}{*}{15} & \cc{cm1$\square$} & 2 & \href{https://cwe.mitre.org/data/definitions/126.html}{126}, \href{https://cwe.mitre.org/data/definitions/476.html}{476} & 87K & \href{https://github.com/mm2/Little-CMS/commit/762d7a64cfd3937a5c1e35f28a34a5558f6788c8}{\cc{762d7a6}} & 2025-05-04 & -- & -- & 32s & 93.0MB \\
\cmidrule{2-14}
 &  &  &  & \cc{mg1$\blacktriangle$} & 1 & \href{https://cwe.mitre.org/data/definitions/121.html}{121} & 352K & \href{https://github.com/cesanta/mongoose/commit/ef8e7419fa704838f8513fd1c6e99363e5dcc182}{\cc{ef8e741}} & 2025-02-02 & 470 & 14 & 17s & 5.5MB \\
\rowcolor{gray!15}  &  &  &  & \cc{mg2$\blacktriangle$} & 1 & \href{https://cwe.mitre.org/data/definitions/125.html}{125} & 352K & \href{https://github.com/cesanta/mongoose/commit/ef8e7419fa704838f8513fd1c6e99363e5dcc182}{\cc{ef8e741}} & 2025-02-02 & 416 & 13 & 17s & 5.5MB \\
 &  &  &  & \cc{mg3$\blacktriangle$} & 0 & -- & 403K & \href{https://github.com/cesanta/mongoose/commit/2df53c3d27b9ae54b1c08b6c3c3cc660a49fa4a2}{\cc{2df53c3}} & 2024-11-20 & 1,019,782 & 1,234 & 16s & 5.5MB \\
\rowcolor{gray!15}  & \multirow{-4}{*}{\href{https://github.com/cesanta/mongoose}{mongoose}} & \multirow{-4}{*}{Network} & \multirow{-4}{*}{1} & \cc{mg1$\square$} & 1 & \href{https://cwe.mitre.org/data/definitions/121.html}{121}, \href{https://cwe.mitre.org/data/definitions/193.html}{193} & 352K & \href{https://github.com/cesanta/mongoose/commit/ef8e7419fa704838f8513fd1c6e99363e5dcc182}{\cc{ef8e741}} & 2025-02-02 & -- & -- & 17s & 5.5MB \\
\cmidrule{2-14}
 & \href{https://github.com/ntop/nDPI}{ndpi} & Network & 55 & \cc{nd1$\square$} & 0 & -- & 136K & \href{https://github.com/ntop/nDPI/commit/8987a2c184b6768b577a4a83e69aacb2bf69856c}{\cc{8987a2c}} & 2025-06-24 & -- & -- & 105s & 1009.0MB \\
\cmidrule{2-14}
\rowcolor{gray!15}  & \href{https://github.com/openssl/openssl}{openssl} & Crypto & 30 & \cc{os1$\square$} & 0 & -- & 909K & \href{https://github.com/openssl/openssl/commit/5b800192f2f9b7b0d3a8add2117fb1ecdd029684}{\cc{5b80019}} & 2025-05-01 & -- & -- & 182s & 747.9MB \\
\cmidrule{2-14}
 & \href{https://github.com/shadowsocks/shadowsocks-libev}{shadowsocks-libev} & Network & 1 & \cc{ss1$\square$} & 5 & \href{https://cwe.mitre.org/data/definitions/126.html}{126} & 19K & \href{https://github.com/shadowsocks/shadowsocks-libev/commit/9afa3cacf947f910be46b69fc5a7a1fdd02fd5e6}{\cc{9afa3ca}} & 2025-01-20 & -- & -- & 86s & 6.2MB \\
\cmidrule{2-14}
\rowcolor{gray!15}  & \href{https://github.com/systemd/systemd}{systemd} & System & 47 & \cc{sd1$\square$} & 4 & \href{https://cwe.mitre.org/data/definitions/122.html}{122}, \href{https://cwe.mitre.org/data/definitions/415.html}{415}, \href{https://cwe.mitre.org/data/definitions/787.html}{787} & 740K & \href{https://github.com/systemd/systemd/commit/d218ecc7337a4689e7d589df7fd146f4aaab3809}{\cc{d218ecc}} & 2024-12-13 & -- & -- & 71s & 253.9MB \\
\cmidrule{2-14}
 &  &  &  & \cc{ws1$\blacktriangle$} & 1 & \href{https://cwe.mitre.org/data/definitions/787.html}{787} & 4901K & \href{https://github.com/wireshark/wireshark/commit/624c0b1f5c695a2765712f03811b011e3b50003c}{\cc{624c0b1}} & 2025-03-04 & 354 & 9 & 462s & 20.9GB \\
\rowcolor{gray!15}  &  &  &  & \cc{ws2$\blacktriangle$} & 1 & \href{https://cwe.mitre.org/data/definitions/121.html}{121} & 4901K & \href{https://github.com/wireshark/wireshark/commit/624c0b1f5c695a2765712f03811b011e3b50003c}{\cc{624c0b1}} & 2025-03-04 & 560 & 10 & 442s & 20.9GB \\
 &  &  &  & \cc{ws3$\blacktriangle$} & 1 & \href{https://cwe.mitre.org/data/definitions/122.html}{122} & 4902K & \href{https://github.com/wireshark/wireshark/commit/624c0b1f5c695a2765712f03811b011e3b50003c}{\cc{624c0b1}} & 2025-03-04 & 407 & 9 & 473s & 20.9GB \\
\rowcolor{gray!15}  &  &  &  & \cc{ws4$\blacktriangle$} & 1 & \href{https://cwe.mitre.org/data/definitions/126.html}{126} & 4901K & \href{https://github.com/wireshark/wireshark/commit/624c0b1f5c695a2765712f03811b011e3b50003c}{\cc{624c0b1}} & 2025-03-04 & 714 & 9 & 464s & 20.9GB \\
 &  &  &  & \cc{ws5$\blacktriangle$} & 1 & \href{https://cwe.mitre.org/data/definitions/129.html}{129} & 4901K & \href{https://github.com/wireshark/wireshark/commit/624c0b1f5c695a2765712f03811b011e3b50003c}{\cc{624c0b1}} & 2025-03-04 & 617 & 8 & 459s & 20.9GB \\
\rowcolor{gray!15}  &  &  &  & \cc{ws7$\blacktriangle$} & 1 & \href{https://cwe.mitre.org/data/definitions/120.html}{120} & 4901K & \href{https://github.com/wireshark/wireshark/commit/624c0b1f5c695a2765712f03811b011e3b50003c}{\cc{624c0b1}} & 2025-03-04 & 420 & 9 & 457s & 20.9GB \\
 & \multirow{-7}{*}{\href{https://github.com/wireshark/wireshark}{wireshark}} & \multirow{-7}{*}{Network} & \multirow{-7}{*}{47} & \cc{ws1$\square$} & 6 & \makecell[l]{\href{https://cwe.mitre.org/data/definitions/121.html}{121}, \href{https://cwe.mitre.org/data/definitions/122.html}{122}, \href{https://cwe.mitre.org/data/definitions/134.html}{134},\\\href{https://cwe.mitre.org/data/definitions/416.html}{416}, \href{https://cwe.mitre.org/data/definitions/457.html}{457}, \href{https://cwe.mitre.org/data/definitions/680.html}{680}} & 4901K & \href{https://github.com/wireshark/wireshark/commit/624c0b1f5c695a2765712f03811b011e3b50003c}{\cc{624c0b1}} & 2025-03-04 & -- & -- & 492s & 20.9GB \\
\cmidrule{2-14}
\rowcolor{gray!15} \multirow{-32}{*}{\textbf{C}} & \href{https://github.com/tukaani-project/xz}{xz} & Compression & 4 & \cc{xz1$\square$} & 1 & \href{https://cwe.mitre.org/data/definitions/416.html}{416} & 41K & \href{https://github.com/tukaani-project/xz/commit/dd4a1b259936880e04669b43e778828b60619860}{\cc{dd4a1b2}} & 2025-05-23 & -- & -- & 37s & 20.0MB \\
\midrule
 &  &  &  & \cc{cc1$\blacktriangle$} & 1 & \href{https://cwe.mitre.org/data/definitions/400.html}{400}, \href{https://cwe.mitre.org/data/definitions/770.html}{770}, \href{https://cwe.mitre.org/data/definitions/1333.html}{1333} & 75K & \href{https://github.com/apache/commons-compress/commit/0df4a4145516ffcf25f2ff53b759453f405ce966}{\cc{0df4a41}} & 2025-02-10 & 205 & 9 & 113s & 17.6MB \\
\rowcolor{gray!15}  &  &  &  & \cc{cc4$\blacktriangle$} & 1 & \href{https://cwe.mitre.org/data/definitions/22.html}{22}, \href{https://cwe.mitre.org/data/definitions/29.html}{29}, \href{https://cwe.mitre.org/data/definitions/35.html}{35} & 76K & \href{https://github.com/apache/commons-compress/commit/3a645c7e15a344961b5e422397a5e2a088fc0b70}{\cc{3a645c7}} & 2025-06-08 & 166 & 10 & 110s & 17.7MB \\
 &  &  &  & \cc{cc5$\blacktriangle$} & 1 & \href{https://cwe.mitre.org/data/definitions/28.html}{28}, \href{https://cwe.mitre.org/data/definitions/77.html}{77} & 76K & \href{https://github.com/apache/commons-compress/commit/3e70c5064257c9e304645ee872fdd9a863328856}{\cc{3e70c50}} & 2025-06-13 & 163 & 8 & 110s & 17.7MB \\
\rowcolor{gray!15}  &  &  &  & \cc{cc6$\blacktriangle$} & 1 & \href{https://cwe.mitre.org/data/definitions/22.html}{22}, \href{https://cwe.mitre.org/data/definitions/29.html}{29}, \href{https://cwe.mitre.org/data/definitions/35.html}{35} & 76K & \href{https://github.com/apache/commons-compress/commit/3a645c7e15a344961b5e422397a5e2a088fc0b70}{\cc{3a645c7}} & 2025-06-08 & 170 & 10 & 108s & 17.7MB \\
 & \multirow{-5}{*}{\href{https://github.com/apache/commons-compress}{commons-compress}} & \multirow{-5}{*}{Compression} & \multirow{-5}{*}{16} & \cc{cc7$\blacktriangle$} & 1 & \href{https://cwe.mitre.org/data/definitions/22.html}{22}, \href{https://cwe.mitre.org/data/definitions/29.html}{29}, \href{https://cwe.mitre.org/data/definitions/35.html}{35} & 76K & \href{https://github.com/apache/commons-compress/commit/3a645c7e15a344961b5e422397a5e2a088fc0b70}{\cc{3a645c7}} & 2025-06-08 & 244 & 10 & 106s & 17.7MB \\
\cmidrule{2-14}
\rowcolor{gray!15}  & \href{https://github.com/dcm4che/dcm4che}{dcm4che} & Healthcare & 1 & \cc{dc1$\square$} & 0 & -- & 105K & \href{https://github.com/dcm4che/dcm4che/commit/d5b4cd32676cf15ab3e38e4f8cdad48d2b9b5536}{\cc{d5b4cd3}} & 2025-06-11 & -- & -- & 315s & 7.7MB \\
\cmidrule{2-14}
 & \href{https://github.com/dicoogle/dicoogle}{dicoogle} & Healthcare & 1 & \cc{dg1$\square$} & 0 & -- & 21K & \href{https://github.com/dicoogle/dicoogle/commit/347692ad9a08ddfd81be3cff3ab360184bcd7e7e}{\cc{347692a}} & 2025-03-10 & -- & -- & 101s & 25.6MB \\
\cmidrule{2-14}
\rowcolor{gray!15}  & \href{https://github.com/GoogleCloudPlatform/healthcare-data-harmonization}{\shortstack[l]{healthcare-\\data-harmonization}} & Healthcare & 1 & \cc{hc1$\square$} & 0 & -- & 53K & \href{https://github.com/GoogleCloudPlatform/healthcare-data-harmonization/commit/a628c4a310b46e74d00f408a57aff8711c90d5a9}{\cc{a628c4a}} & 2025-06-02 & -- & -- & 80s & 11.2MB \\
\cmidrule{2-14}
 & \href{https://github.com/apache/hertzbeat}{hertzbeat} & Monitoring & 1 & \cc{hb1$\square$} & 0 & -- & 78K & \href{https://github.com/apache/hertzbeat/commit/d077c7221142f794624e0b08aa9d057da556090e}{\cc{d077c72}} & 2025-06-13 & -- & -- & 170s & 349.7MB \\
\cmidrule{2-14}
\rowcolor{gray!15}  & \href{https://github.com/jhy/jsoup}{jsoup} & Document & 2 & \cc{js1$\square$} & 0 & -- & 36K & \href{https://github.com/jhy/jsoup/commit/3b97e9616b96c80b8211a2fb7358c350b491c76e}{\cc{3b97e96}} & 2025-06-30 & -- & -- & 79s & 8.2MB \\
\cmidrule{2-14}
 & \href{https://github.com/apache/logging-log4j2}{log4j2} & Logging & 1 & \cc{lj1$\blacktriangle$} & 1 & \href{https://cwe.mitre.org/data/definitions/20.html}{20}, \href{https://cwe.mitre.org/data/definitions/917.html}{917} & 54K & \href{https://github.com/apache/logging-log4j2/commit/f1a0cac60f1e41347c9bced7c1470be488840344}{\cc{f1a0cac}} & 2013-07-18 & 535 & 17 & 96s & 8.4MB \\
\cmidrule{2-14}
\rowcolor{gray!15}  &  &  &  & \cc{pb1$\blacktriangle$} & 1 & \href{https://cwe.mitre.org/data/definitions/28.html}{28}, \href{https://cwe.mitre.org/data/definitions/77.html}{77} & 167K & \href{https://github.com/apache/pdfbox/commit/afd3ea77c9cecc5a85b815e202bc84d6dd7a2b6e}{\cc{afd3ea7}} & 2025-06-11 & 455 & 12 & 135s & 7.7MB \\
 & \multirow{-2}{*}{\href{https://github.com/apache/pdfbox}{pdfbox}} & \multirow{-2}{*}{Document} & \multirow{-2}{*}{6} & \cc{pb1$\square$} & 8 & \makecell[l]{\href{https://cwe.mitre.org/data/definitions/611.html}{611}, \href{https://cwe.mitre.org/data/definitions/789.html}{789}, \href{https://cwe.mitre.org/data/definitions/834.html}{834},\\\href{https://cwe.mitre.org/data/definitions/835.html}{835}, \href{https://cwe.mitre.org/data/definitions/918.html}{918}} & 167K & \href{https://github.com/apache/pdfbox/commit/afd3ea77c9cecc5a85b815e202bc84d6dd7a2b6e}{\cc{afd3ea7}} & 2025-06-11 & -- & -- & 129s & 7.7MB \\
\cmidrule{2-14}
\rowcolor{gray!15}  &  &  &  & \cc{po1$\blacktriangle$} & 2 & \href{https://cwe.mitre.org/data/definitions/20.html}{20}, \href{https://cwe.mitre.org/data/definitions/121.html}{121}, \href{https://cwe.mitre.org/data/definitions/918.html}{918} & 433K & \href{https://github.com/apache/poi/commit/c784266438a28d8e1868242bc261961b894fe3c8}{\cc{c784266}} & 2025-06-17 & 318 & 17 & 216s & 14.4MB \\
 & \multirow{-2}{*}{\href{https://github.com/apache/poi}{poi}} & \multirow{-2}{*}{Document} & \multirow{-2}{*}{17} & \cc{po1$\square$} & 5 & \makecell[l]{\href{https://cwe.mitre.org/data/definitions/20.html}{20}, \href{https://cwe.mitre.org/data/definitions/35.html}{35}, \href{https://cwe.mitre.org/data/definitions/382.html}{382}, \href{https://cwe.mitre.org/data/definitions/695.html}{695},\\\href{https://cwe.mitre.org/data/definitions/770.html}{770}, \href{https://cwe.mitre.org/data/definitions/789.html}{789}, \href{https://cwe.mitre.org/data/definitions/834.html}{834}} & 433K & \href{https://github.com/apache/poi/commit/c784266438a28d8e1868242bc261961b894fe3c8}{\cc{c784266}} & 2025-06-17 & -- & -- & 206s & 14.4MB \\
\cmidrule{2-14}
\rowcolor{gray!15} \multirow{-16}{*}{\textbf{Java}} & \href{https://github.com/apache/tika}{tika} & Document & 9 & \cc{tk6$\blacktriangle$} & 1 & \href{https://cwe.mitre.org/data/definitions/407.html}{407}, \href{https://cwe.mitre.org/data/definitions/834.html}{834} & 188K & \href{https://github.com/apache/tika/commit/2d199aa0da8421f88bf424d84c106d092751e46b}{\cc{2d199aa}} & 2025-06-03 & 482 & 11 & 150s & 61.3MB \\
\bottomrule
\end{tabular}
\end{threeparttable}
}
\end{table*}
